# Supplementary material for: Semantic Self-adaptation: Enhancing Generalization with a Single Sample
Source: arXiv:2208.05788 source file (2023-12-13)
Supplement: Supplementary file 1 [file supp_sota.tex]

%In \cref{table:sota_cmp_add}, we compare our method to the more recent approaches: RobustNet \citep{Choi:2021:Rob} and FSDR \citep{Huang:2021:FSD}. \citet{Choi:2021:Rob} disentangle domain-specific and domain-invariant properties from higher-order statistics of the feature representation by using an instance selective whitening loss. FSDR \citep{Huang:2021:FSD} randomizes images in the frequency space by keeping domain-invariant frequency components and varying the domain-sensitive frequency components.

For a fair comparison with RobustNet \citep{Choi:2021:Rob}, we trained a DeepLabv3+ model with the output stride of 16 in contrast to the output stride of 8 used by default (\eg, in \cref{table:recent_arch}).
We also remark that FSDR used the target domains for hyperparameter tuning and model selection, which gives it a clear advantage.\footnote{\href{https://github.com/jxhuang0508/FSDR/issues/2\#issuecomment-910089417}{https://github.com/jxhuang0508/FSDR/issues/2\#issuecomment-910089417}} Nonetheless, we outperform FSDR in terms of IoU on two out of three target domains using ResNet-101 backbone.
Remarkably, our baseline training schedule and data augmentation alone already reach the accuracy of RobustNet without any additional regularization or changes to the model architecture.
Our IaBN with Seg-TTT further improve over these results by significant margins (more than 8\% IoU) across all tested target domains.

\begin{table}[!t]
  \caption{\textit{Mean IoU (\%) comparison to state-of-the-art domain generalization methods} for both source domains (\gta, \synthia) as well as three target domains (Cityscapes, Mapillary, BDD). We compare to RobustNet \citep{Choi:2021:Rob} and FSDR \citep{Huang:2021:FSD}. $(^\ddagger)$ and $(^{\dagger\dagger})$ denote the use of FCN~\citep{Long:2015:FCN} and DeepLabv3+ ~\citep{Chen:2018:ECA} architectures, respectively.}
  \label{table:sota_cmp_add}
  \smallskip
  \centering
  \footnotesize
  \setlength\tabcolsep{4pt}

\begin{tabularx}{\linewidth}{@{}lXl@{\hspace{0.3mm}}ll@{\hspace{0.3mm}}ll@{\hspace{0.3mm}}l@{\hspace{0.6em}}l@{\hspace{0.3mm}}ll@{\hspace{0.3mm}}ll@{\hspace{0.3mm}}l@{}}
\toprule
& \multirow{2}{*}{Method} & \multicolumn{6}{@{}c@{\hspace{1em}}}{\textit{Backbone: ResNet-50}} & \multicolumn{6}{@{\hspace{1em}}c@{}}{\textit{Backbone: ResNet-101}} \\
\cmidrule(l{1em}r@{2em}){3-8} \cmidrule(lr){9-14}
& & \multicolumn{2}{c}{CS} & \multicolumn{2}{c}{Mapillary} & \multicolumn{2}{c}{BDD} & \multicolumn{2}{c}{CS}  & \multicolumn{2}{c}{Mapillary} & \multicolumn{2}{c}{BDD} \\
\midrule
\multirow{5}{*}{\rotatebox[origin=c]{90}{\textit{\gta}}}
& No Adapt & 28.95 & \multirow{2}{*}{$\uparrow$\textit{7.63}} & 28.18 & \multirow{2}{*}{$\uparrow$\textit{12.15}}   & 25.14 & \multirow{2}{*}{$\uparrow$\textit{10.06}} & & \multirow{2}{*}{--} & & \multirow{2}{*}{--} & & \multirow{2}{*}{--} \\
& RobustNet$^{\dagger\dagger}$ & 36.58 & & 40.33 & & 35.20 & & & & & & &  \\[6pt]

& No Adapt & 37.75 & \multirow{2}{*}{$\uparrow$\textit{8.36}} & 40.36 & \multirow{2}{*}{$\uparrow$\textit{9.17}}   & 33.70 & \multirow{2}{*}{$\uparrow$\textit{8.05}} & & \multirow{2}{*}{--} & & \multirow{2}{*}{--} & & \multirow{2}{*}{--} \\
& Ours$^{\dagger\dagger}$ & \textbf{46.11} & & \textbf{49.53} & & \textbf{41.75} & & & & & & &  \\
%& No Adapt & 36.28 & \multirow{2}{*}{$\uparrow$\textit{9.74}} & 40.94 & \multirow{2}{*}{$\uparrow$\textit{6.86}}   & 34.51 & \multirow{2}{*}{$\uparrow$\textit{5.85}} & & \multirow{2}{*}{--} & & \multirow{2}{*}{--} & & \multirow{2}{*}{--} \\
%& Ours$^{\dagger\dagger}$ & \textbf{46.02} & & \textbf{47.80} & & \textbf{40.36} & & & & & & &  \\
\midrule
\multirow{5}{*}{\rotatebox[origin=c]{90}{\textit{\gta}}}
& No Adapt  & & \multirow{2}{*}{--} & & \multirow{2}{*}{--} & & \multirow{2}{*}{--} & 33.4 & \multirow{2}{*}{$\uparrow$\textit{11.4}} & 27.9 & \multirow{2}{*}{$\uparrow$\textit{15.5}} & 27.3 & \multirow{2}{*}{$\uparrow$\textit{13.9}} \\
& FSDR$^\ddagger$ & & & & & & & 44.8 & & 43.4 & & \textbf{41.2} & \\[6pt]

& No Adapt & 30.95 & \multirow{2}{*}{$\uparrow$\textit{14.18}}  & 34.56 & \multirow{2}{*}{$\uparrow$\textit{12.93}} & 28.52 & \multirow{2}{*}{$\uparrow$\textit{11.09}} & 32.90 & \multirow{2}{*}{$\uparrow$\textit{14.09}} & 36.00 & \multirow{2}{*}{$\uparrow$\textit{11.49}} & 32.54 & \multirow{2}{*}{$\uparrow$\textit{7.67}} \\
& Ours & \textbf{45.13} & & \textbf{47.49} & & \textbf{39.61} & & \textbf{46.99} & & \textbf{47.49} & & 40.21 & \\
\midrule
\multirow{5}{*}{\rotatebox[origin=c]{90}{\textit{\synthia}}}
& No Adapt  & & \multirow{2}{*}{--} & & \multirow{2}{*}{--} & & \multirow{2}{*}{--} & - &  & - &  & - &  \\
& FSDR$^\ddagger$ & & & & & & & 40.8 & & 39.6 & & \textbf{37.4} & \\[6pt]

& No Adapt & 31.83 & \multirow{2}{*}{$\uparrow$\textit{9.77}} & 33.41 & \multirow{2}{*}{$\uparrow$\textit{7.80}} & 24.30 & \multirow{2}{*}{$\uparrow$\textit{9.05}} & 37.25 & \multirow{2}{*}{$\uparrow$\textit{5.07}} & 36.84 & \multirow{2}{*}{$\uparrow$\textit{4.36}} & 29.32 & \multirow{2}{*}{$\uparrow$\textit{3.95}} \\
& Ours & \textbf{41.60} & & \textbf{41.21} & & \textbf{33.35} & & \textbf{42.32} & & \textbf{41.20} & & 33.27 & \\
\bottomrule
\end{tabularx}
\end{table}
