# Supplementary material for: Semantic Self-adaptation: Enhancing Generalization with a Single Sample
Source: arXiv:2208.05788 source file (2023-12-13)

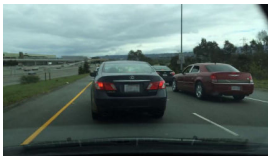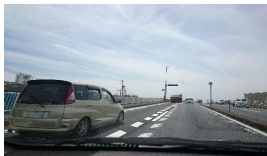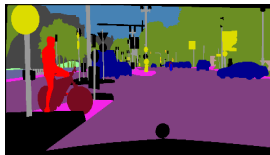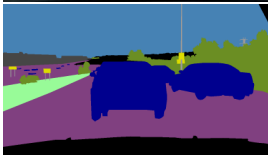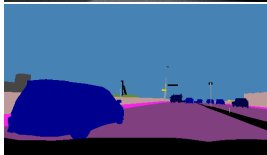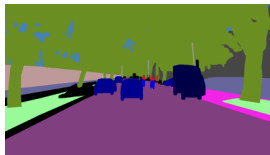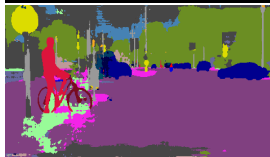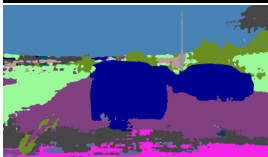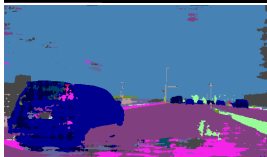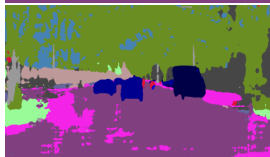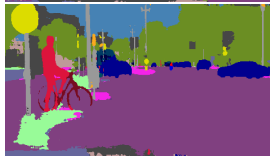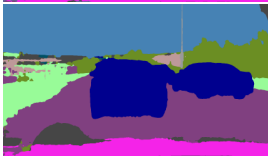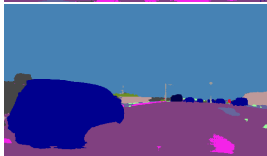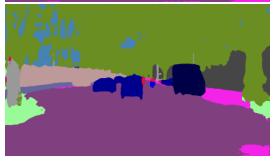

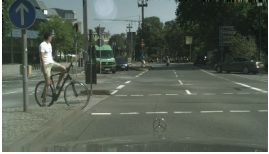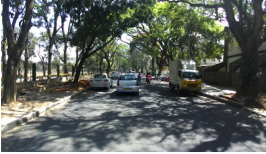

Supplement: Supplementary file 3 [file fresults_fig_gta101_im.pdf]
